# Supplementary material for: Measurement of the W boson mass
Source: arXiv:2109.01113 source file (2022-01-14)
Supplement: Supplementary file 1 [file appendix.tex]

% ===============================================================================
% Purpose: appendix to the standard template: standard symbol alises from Ulrik
% Author: Tomasz Skwarnicki
% Created on: 2009-09-24
% ===============================================================================

%{\noindent\normalfont\bfseries\Large Appendices}
\section*{Appendices}

\appendix

\section{Example section on material to appear in appendix of paper}
\label{sec:App1}
Here we can put material that will appear on the arXiv and journal version.
